# Supplementary material for: Watermarking Recommender Systems
Source: arXiv:2407.21034 source file (2024-09-30)
Supplement: Supplementary file 1 [file appendix.tex]

\newpage
\appendix

\begin{table*}[h]
\caption{Watermark validity in percentage on the distilled SASRec model.}
\vspace{-1.5em}
\begin{center}
 \begin{tabular}{|c|c|c|c|c|c|c|c|c|c|c|c|c|} 
 \hline
 Dataset & Method & $n$ & R@1 & R@5 & R@10 & R@20 & R@100 & N@1 & N@5 & N@10 & N@20 & N@100 \\
    \hline
   \multirow{8}{*}{ML-1M} & \multirow{4}{*}{cold} & 2 & 100.00 & 100.00 & 100.00 & 100.00 & 100.00 & 100.00 & 100.00 & 100.00 & 100.00 & 100.00 \\
     \cline{3-3}
 &  & 5 & 73.69 & 73.69 & 73.69 & 73.69 & 100.00 & 73.69 & 73.69 & 73.69 & 73.69 & 78.70 \\
  \cline{3-3}
 &  & 10 & 22.51 & 57.12 & 57.12 & 67.36 & 100.00 & 22.51 & 42.21 & 42.21 & 44.97 & 50.73 \\
  \cline{3-3}
  &  & 20 & 15.61 & 48.07 & 57.15 & 66.17 & 70.78 & 15.61 & 30.96 & 33.99 & 36.47 & 37.43 \\
 \cline{2-13}
 & \multirow{4}{*}{pop} & 2 & 0.00 & 0.00 & 100.00 & 100.00 & 100.00 & 0.00 & 0.00 & 33.33 & 33.33 & 33.33 \\
  \cline{3-3}
   & & 5 & 0.00 & 0.00 & 0.00 & 50.59 & 75.58 & 0.00 & 0.00 & 0.00 & 12.65 & 17.85 \\
 \cline{3-3}
  & & 10 & 9.89 & 42.71 & 55.03 & 66.70 & 100.00 & 9.89 & 26.44 & 30.15 & 32.80 & 38.76 \\
  \cline{3-3}
  & & 20 & 11.75 & 42.13 & 64.22 & 69.38 & 100.00 & 11.75 & 28.79 & 35.86 & 37.21 & 42.48 \\
  \hline
   \multirow{8}{*}{ML-20M} & \multirow{4}{*}{cold} & 2 & 100.00 & 100.00 & 100.00 & 100.00 & 100.00 & 100.00 & 100.00 & 100.00 & 100.00 & 100.00 \\
     \cline{3-3}
 & & 5 & 0.00 & 100.00 & 100.00 & 100.00 & 100.00 & 0.00 & 52.05 & 52.05 & 52.05 & 52.05 \\
  \cline{3-3}
 &  & 10 & 9.53 & 19.05 & 28.88 & 64.10 & 100.00 & 9.53 & 14.29 & 17.57 & 26.22 & 32.95 \\
  \cline{3-3}
  &  & 20 & 0.00 & 15.29 & 35.71 & 48.28 & 89.72 & 0.00 & 7.16 & 13.62 & 16.94 & 24.91 \\
 \cline{2-13}
 & \multirow{4}{*}{pop} & 2 & 0.00 & 0.00 & 0.00 & 0.00 & 0.00 & 0.00 & 0.00 & 0.00 & 0.00 & 0.00 \\
  \cline{3-3}
 & & 5 & 0.00 & 23.49 & 23.49 & 23.49 & 23.49 & 0.00 & 10.12 & 10.12 & 10.12 & 10.12 \\
 \cline{3-3}
 & & 10 & 0.00 & 46.30 & 87.99 & 87.99 & 87.99 & 0.00 & 24.57 & 37.97 & 37.97 & 37.97 \\
  \cline{3-3}
 & & 20 & 5.39 & 36.87 & 58.10 & 89.78 & 100.00 & 5.39 & 20.92 & 27.42 & 35.52 & 37.10 \\
    \hline
   \multirow{8}{*}{Steam} & \multirow{4}{*}{cold} & 2 & 100.00 & 100.00 & 100.00 & 100.00 & 100.00 & 100.00 & 100.00 & 100.00 & 100.00 & 100.00 \\
     \cline{3-3}
 &  & 5 & 0.00 & 100.00 & 100.00 & 100.00 & 100.00 & 0.00 & 56.78 & 56.78 & 56.78 & 56.78 \\
  \cline{3-3}
 &  & 10 & 0.00 & 75.98 & 75.98 & 87.95 & 100.00 & 0.00 & 46.38 & 46.38 & 49.15 & 50.99 \\
  \cline{3-3}
  &  & 20 & 4.27 & 47.48 & 52.46 & 61.58 & 66.96 & 4.27 & 26.63 & 28.40 & 30.68 & 31.68 \\
 \cline{2-13}
 & \multirow{4}{*}{pop} & 2 & 0.00 & 100.00 & 100.00 & 100.00 & 100.00 & 0.00 & 38.69 & 38.69 & 38.69 & 38.69 \\
  \cline{3-3}
   & & 5 & 0.00 & 22.96 & 22.96 & 22.96 & 22.96 & 0.00 & 14.48 & 14.48 & 14.48 & 14.48 \\
 \cline{3-3}
  & & 10 & 21.73 & 78.17 & 89.79 & 89.79 & 100.00 & 21.73 & 54.17 & 57.83 & 57.83 & 59.62 \\
  \cline{3-3}
  & & 20 & 5.31 & 14.72 & 41.67 & 53.75 & 79.07 & 5.31 & 9.11 & 18.22 & 21.39 & 26.23 \\
    \hline
\multirow{8}{*}{Beauty} & \multirow{4}{*}{cold} & 2 & 100.00 & 100.00 & 100.00 & 100.00 & 100.00 & 100.00 & 100.00 & 100.00 & 100.00 & 100.00 \\
  \cline{3-3}
 &  & 5 & 28.78 & 100.00 & 100.00 & 100.00 & 100.00 & 28.78 & 68.39 & 68.39 & 68.39 & 68.39 \\
  \cline{3-3}
 &  & 10 & 33.87 & 100.00 & 100.00 & 100.00 & 100.00 & 33.87 & 75.59 & 75.59 & 75.59 & 75.59 \\
  \cline{3-3}
  &  & 20 & 36.44 & 89.54 & 100.00 & 100.00 & 100.00 & 36.44 & 66.74 & 69.90 & 69.90 & 69.90 \\
 \cline{2-13}
 & \multirow{4}{*}{pop} & 2 & 100.00 & 100.00 & 100.00 & 100.00 & 100.00 & 100.00 & 100.00 & 100.00 & 100.00 & 100.00 \\
  \cline{3-3}
   & & 5 & 74.68 & 100.00 & 100.00 & 100.00 & 100.00 & 74.68 & 90.66 & 90.66 & 90.66 & 90.66 \\
 \cline{3-3}
  & & 10 & 69.88 & 91.05 & 100.00 & 100.00 & 100.00 & 69.88 & 83.24 & 86.22 & 86.22 & 86.22 \\
  \cline{3-3}
  & & 20 & 21.42 & 88.36 & 100.00 & 100.00 & 100.00 & 21.42 & 59.35 & 63.50 & 63.50 & 63.50 \\
    \hline
\end{tabular}
\label{table:distillation_sasrec}
\end{center}
\vspace{-1em}
\end{table*}

\section{Experiment on SASRec}
\label{appendix:sasrec}
\autoref{table:distillation_sasrec} shows the watermark validity after distillation on SASRec.

\begin{table}[h]
\caption{Recall@1 in percentage of the watermark at different watermark lengths $n$ on SASRec.}
\vspace{-1.5em}
\begin{center}
 \begin{tabular}{|c|c|c|c|c|c|} 
 \hline
  \multirow{2}{*}{Dataset} & \multirow{2}{*}{Method} & \multicolumn{4}{c|}{$n$} \\
 \cline{3-6}
   & & 2 & 5 & 10 & 20 \\
  \hline
 \multirow{2}{*}{ML-1M} & cold & 100.00 & 100.00 & 100.00 & 100.00 \\
   \cline{2-2}
 & pop & 100.00 & 100.00 & 100.00 & 100.00 \\
  \hline
   \multirow{2}{*}{ML-20M} & cold & 100.00 & 100.00 & 100.00 & 100.00 \\
   \cline{2-2}
 & pop & 100.00 & 100.00 & 100.00 & 100.00 \\
 \hline
 \multirow{2}{*}{Steam} & cold & 100.00 & 100.00 & 100.00 & 100.00 \\
   \cline{2-2}
 & pop & 100.00 & 100.00 & 100.00 & 100.00 \\
  \hline
  \multirow{2}{*}{Beauty} & cold & 100.00 & 100.00 & 100.00 & 100.00  \\
   \cline{2-2}
 & pop & 100.00 & 100.00 & 100.00 & 100.00 \\
 \hline
\end{tabular}
\label{table:validity sasrec}
\end{center}
\vspace{-1em}
\end{table}
